# Supplementary material for: Optically heralded microwave photons
Source: arXiv:2210.10739 source file (2022-10-19)

**a**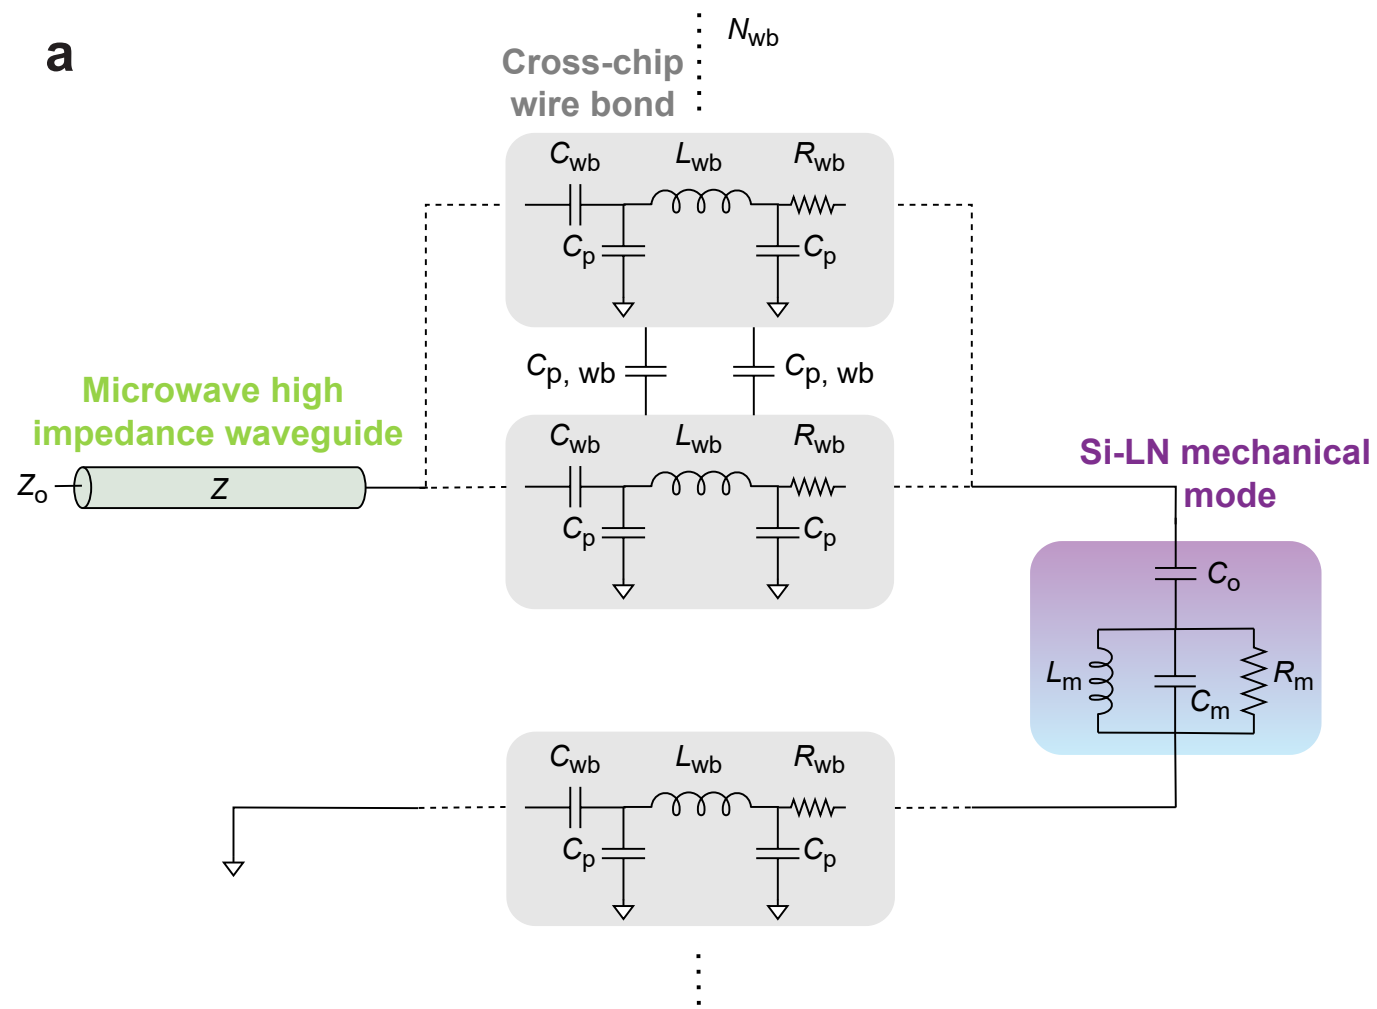**b**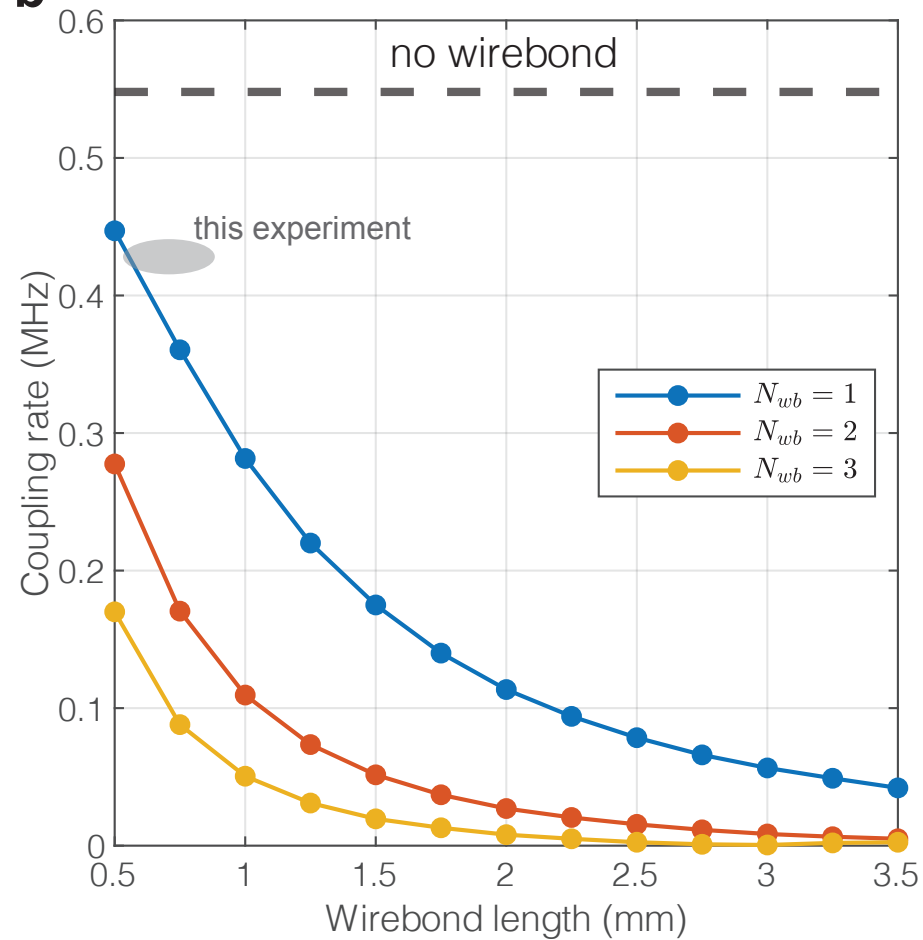

Supplement: Supplementary file 1 [file SI_XCWB_20220915_v3.pdf]
